# Supplementary material for: Experimental determination of superexchange energy from two-hole spectra
Source: arXiv:2107.09181 source file (2021-07-19)
Supplement: Supplementary file 1 [file LevyG2021_SM.pdf]

# Supplemental Materials

## Experimental determination of superexchange energy from two-hole spectra

Giorgio Levy,<sup>1,2,\*</sup> Maayan Yaari,<sup>3</sup> Tom Z. Regier,<sup>4</sup> and Amit Keren<sup>3</sup>

<sup>1</sup>Quantum Matter Institute, University of British Columbia, Vancouver, British Columbia V6T 1Z4, Canada

<sup>2</sup>Department of Physics and Astronomy, University of British Columbia, Vancouver, British Columbia V6T 1Z1, Canada

<sup>3</sup>Department of Physics, Technion - Israel Institute of Technology, Haifa, 3200003, Israel

<sup>4</sup>Canadian Light Source Inc., 44 Innovation Boulevard, Saskatoon, SK, S7N 2V3, Canada

(Dated: July 12, 2021)

### Near valence-band photoemission spectroscopy

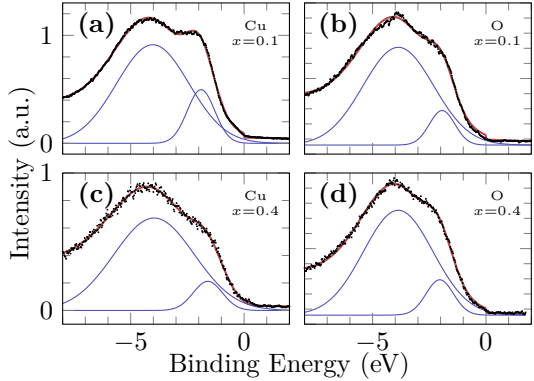

FIG. 1. Near valence band photoemission spectra in **CL123** plotted as black dots for photon energies far from the resonant behavior. The red curves shows the best fit to the data with a model including two Gaussian profiles (blue curves) multiplied by a Fermi-Dirac distribution and a Shirley-type background (red lines). The spectra at energies lower than the Cu-2p ( $h\nu=924$  eV) [O-1s ( $h\nu=528$  eV)] absorption edge for the  $x=0.1$  composition, are shown in panels (a) [(b)]; for  $x=0.4$ , in panel (c) [(d)].

The photoemission spectra at energies smaller than the absorption for Cu-2p and O-1s in the binding energy region between  $BE=-8 - 1$  eV is described by two peaks

| Composition | PE (eV) | $BE$ (eV)        | $BE$ (eV)        |
|-------------|---------|------------------|------------------|
| $h\nu$      | $x$     | Cu-3d            | O-2p             |
| 924         | 0.1     | $-1.90 \pm 0.05$ | $-4.03 \pm 0.05$ |
| 528         | 0.1     | $-1.93 \pm 0.05$ | $-3.86 \pm 0.05$ |
| 924         | 0.4     | $-1.60 \pm 0.05$ | $-3.96 \pm 0.05$ |
| 528         | 0.4     | $-2.04 \pm 0.05$ | $-3.87 \pm 0.05$ |
| Average     | 0.1     | $-1.92 \pm 0.04$ | $-3.94 \pm 0.07$ |
| Average     | 0.4     | $-1.8 \pm 0.1$   | $-3.92 \pm 0.04$ |

TABLE I. Binding energy ( $BE$ ) of the two spectral features assigned to Cu-3d and O-2p states for photon energies ( $PE$ )  $h\nu=924$  and  $528$  eV and compositions  $x=0.1$ . The last two rows show the binding energy averages for a given photon energy.

centered at  $BE \approx -4$  eV and  $BE \approx -2$  eV. The panels (a) and (b) in Figure 1 shows the spectra for  $x=0.1$  composition acquired with a light beam of energy  $h\nu=924$  eV and  $h\nu=528$ ; panels (c) and (d) for  $x=0.4$ . To determine their position, we have fit them with a model composed of two peaks described by Gaussian lineshapes multiplied by a Fermi-Dirac function plus a Shirley-type background. Table I summarizes the determined binding energies of the corresponding features. The peak centered in average at  $BE=-3.9 \pm 0.1$  eV is assigned to the Cu-3d states, and the peak around  $BE=-1.9 \pm 0.1$  eV to O-2p states.

### Slater-Condon Parameters

The singlets assigned in the two-hole spectra are related to the multipole expansion of the Coulomb potential in the subspace determined by the total angular momentum  $L$  [1]. For a  $d^8$  configuration, the relation between the multipoles  $F^0$ ,  $F^2$ , and  $F^4$  and the relative energies of the multiplets  $^1S$ ,  $^1D$ ,  $^1G$  can be written in matrix form:

$$\begin{pmatrix} F^0 \\ F^2 \\ F^4 \end{pmatrix} = \begin{pmatrix} -\frac{3}{25} & \frac{2}{5} & \frac{18}{25} \\ \frac{1}{35} & -\frac{5}{49} & \frac{18}{245} \\ \frac{1}{175} & \frac{2}{245} & -\frac{17}{1225} \end{pmatrix} \begin{pmatrix} E(^1S) \\ E(^1D) \\ E(^1G) \end{pmatrix}$$

Based on the energies for the singlets  $^1S$ ,  $^1D$ , and  $^1G$  extracted from the fits to the two-hole spectra, the following multipoles values are obtained for  $x=0.1$ :  $U_d^{x01} \equiv F_{Cu}^0=5.91 \pm 0.03$  eV,  $F_{Cu}^2=18.83 \pm 0.07$  eV,  $F_{Cu}^4=0.4 \pm 0.1$  eV. And for  $x=0.4$ , the multipoles values are:  $F_{Cu}^0=5.76 \pm 0.04$  eV,  $F_{Cu}^2=19.57 \pm 0.06$  eV,  $F_{Cu}^4=0.2 \pm 0.1$  eV.

For  $p^4$  configuration in Oxygen, the relation between the Coulomb multipoles  $F^0$  and  $F^2$  and the relative energy of the singlets  $^1S$  and  $^1D$  is

$$\begin{pmatrix} F^0 \\ F^2 \end{pmatrix} = \frac{1}{9} \begin{pmatrix} -1 & 10 \\ 1 & -1 \end{pmatrix} \begin{pmatrix} E(^1S) \\ E(^1D) \end{pmatrix}$$

In O- $p^4$  configuration, We obtain the following values for  $x=0.1$ :  $U_p^{x01} \equiv F^0=4.18 \pm 0.02$  eV and  $F^2=5.9 \pm 0.2$  eV; for  $x=0.4$ :  $F^0=4.47 \pm 0.06$  eV and  $F^2=7.7 \pm 0.1$  eV.

### Superexchange interaction $J$

Following Pavarini *et al.* [2], we determine the superexchange interaction between two adjacent Cu atoms mediated by an intermediate Oxygen as the energy difference of the triplet with respect to the singlet lowest energy state. In addition to the O and Cu on-site energy difference ( $\Delta$ ), the charge transfer hopping  $t_{pd}$ , and the Coulomb repulsion for two electrons on Cu-3d level ( $U_d$ ), we include the Coulomb interaction of two electrons in O-2p level ( $U_p$ ). Therefore, the Hamiltonian matrix in the triplet subspace is:

$$H_T = \begin{pmatrix} U_d + \Delta & t_{pd} & 0 \\ t_{pd} & U_p & t_{pd} \\ 0 & t_{pd} & U_d + \Delta \end{pmatrix},$$

and in the single subspace is:

$$H_S = \begin{pmatrix} U_p & 0 & \sqrt{2}t_{pd} & 0 & 0 & 0 \\ 0 & U_p & 0 & \sqrt{2}t_{pd} & 0 & 0 \\ \sqrt{2}t_{pd} & 0 & U_d + \Delta & 0 & -t_{pd} & -\sqrt{2}t_{pd} \\ 0 & \sqrt{2}t_{pd} & 0 & U_d + \Delta & t_{pd} & \sqrt{2}t_{pd} \\ 0 & 0 & -t_{pd} & t_{pd} & U_d + U_p & 0 \\ 0 & 0 & -\sqrt{2}t_{pd} & \sqrt{2}t_{pd} & 0 & 2(U_d + \Delta) \end{pmatrix}.$$

### Determination of $J$

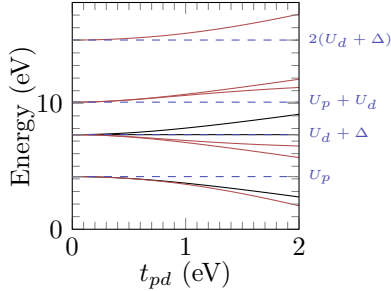

FIG. 2. **The determination of the superexchange energy  $J$**  variation with the charge transfer hopping  $t_{pd}$ . The energy spectrum for states in a singlet (red lines) and triplet (black lines) configuration were calculated numerically using the charge transfer gap  $\Delta_{Cu}$ , the on-site Coulomb repulsion on Cu-3d ( $U_d$ ) and on O-2p ( $U_p$ ) levels as extracted for  $x=0.1$  composition. These values are obtained from the analysis of the absorption and the two-hole spectra (see main text). The blue dashed lines represent the energy spectrum for  $t_{pd} = 0$ . We define the superexchange energy  $J$  as the energy different between the lowest eigenvalues for the triplet with respect to the singlet state.

The superexchange energy  $J$  is numerically calculated from the energy spectrum for the triplet and singlet configurations (see Fig. 2). Its value is obtained by subtracting the lowest energy value for the triplet state from the singlet ground state.

---

\* E-mail: [levyg@phas.ubc.ca](mailto:levyg@phas.ubc.ca)

- [1] J. Griffith, *The theory of transition-metal ions* (Cambridge University Press, 1961).
- [2] E. Pavarini, E. Koch, R. Scalettar, and R. Martin, eds., *The Physics of Correlated Insulators, Metals, and Superconductors*, Schriften des Forschungszentrums Jülich Reihe Modeling and Simulation, Vol. 7 (Forschungszentrum Jülich GmbH Zentralbibliothek, Verlag, Jülich, 2017) p. 450 p.
